# Supplementary material for: Rules for Phase Shifts of Quantum Oscillations in Topological Nodal-line Semimetals
Source: arXiv:1801.05709 source file (2018-03-03)
Supplement: Supplementary file 1 [file oscillation_NL_prl_supp_20180219.pdf]

# Supplemental Material for "Rules for Phase Shifts of Quantum Oscillations in Topological Nodal-line Semimetals"

Cequn Li,[1,2,3] C. M. Wang,[1,2,4] Bo Wan,[5,1] Xiangang Wan,[5] Hai-Zhou Lu,[1,2,*] and X. C. Xie[6,7]

[1]*Shenzhen Institute for Quantum Science and Engineering and Department of Physics, Southern University of Science and Technology, Shenzhen 518055, China*
[2]*Shenzhen Key Laboratory of Quantum Science and Engineering, Shenzhen 518055, China*
[3]*Department of Physics, The Pennsylvania State University, University Park, Pennsylvania 16802, USA*
[4]*School of Physics and Electrical Engineering, Anyang Normal University, Anyang 455000, China*
[5]*National Laboratory of Solid State Microstructures, Collaborative Innovation Center of Advanced Microstructures, School of Physics, Nanjing University, Nanjing 210093, P. R. China*
[6]*International Center for Quantum Materials, School of Physics, Peking University, Beijing 100871, China*
[7]*Collaborative Innovation Center of Quantum Matter, Beijing 100871, China*

(Dated: February 26, 2018)

In this Supplemental Material, we present the calculations for those in the list of contents.

## CONTENTS

S1. A survey of the phase shifts of the quantum oscillation in experiments S1

S2. The $\pi$ Berry phase around the nodal line S1

S3. Landau bands S2

S4. Magnetoconductivities in and out of the nodal-ring plane S4
A. Conductivity $\sigma_{zz}$ out of the nodal-ring plane S4
B. Conductivity $\sigma_{yy}$ in the nodal-ring plane S4
C. Hall conductivity $\sigma_{xy}$ in the nodal-ring plane S5

S5. Scattering matrix elements S5

S6. The transport time $\tau_{+\nu}^{k_x,k_z}$ S6

S7. Relation about $\Lambda_{\mu,s_2}^{\nu,s_1}$ S6

S8. Phase shifts in $B_{||}$ S7

S9. Phase shift of trivial bands S7

References S8

## S1. A SURVEY OF THE PHASE SHIFTS OF THE QUANTUM OSCILLATION IN EXPERIMENTS

See Table I for a survey of the phase shifts of SdH and dHvA oscillations in nodal-line semimetals collected from the recent experiments.

* Corresponding author. luhz@sustc.edu.cn

## S2. THE $\pi$ BERRY PHASE AROUND THE NODAL LINE

To evaluate the Berry phase of this nodal line semimetal, we add a term related to $\tau_2$ to the previous Hamiltonian

$$H' = \left\{\left[\frac{\hbar^2(k_x^2+k_y^2)}{2m} - u\right]\tau_3 + \lambda k_z \tau_1 + \frac{\Delta}{2}\tau_2\right\} \otimes \sigma_0. \tag{S1}$$

The Hamiltonian of the nodal line semimetals could be obtained by setting $\Delta \to 0$. The eigenenergies of the above Hamiltonian are $E_{\mathbf{k}}^{\pm} = \pm\varepsilon_{\mathbf{k}} = \pm\sqrt{a^2+b^2+\Delta^2/4}$ with $a = \hbar^2(k_x^2+k_y^2)/(2m) - u$ and $b = \lambda k_z$. The eigenstate for $E_{\mathbf{k}}^{+}$ is

$$\psi_{\mathbf{k}}^{+} = C_+ \begin{bmatrix} 0 \\ \frac{b-i\Delta/2}{\varepsilon_{\mathbf{k}}-a} \\ 0 \\ 1 \end{bmatrix} \text{ or } C_+ \begin{bmatrix} \frac{b-i\Delta/2}{\varepsilon_{\mathbf{k}}-a} \\ 0 \\ 1 \\ 0 \end{bmatrix}, \tag{S2}$$

and the eigenstate for $E_{\mathbf{k}}^{-}$ is

$$\psi_{\mathbf{k}}^{-} = C_- \begin{bmatrix} 0 \\ \frac{i\Delta/2-b}{\varepsilon_{\mathbf{k}}+a} \\ 0 \\ 1 \end{bmatrix} \text{ or } C_- \begin{bmatrix} \frac{i\Delta/2-b}{\varepsilon_{\mathbf{k}}+a} \\ 0 \\ 1 \\ 0 \end{bmatrix}. \tag{S3}$$

Here

$$C_{\pm} = \frac{\sqrt{2}}{2}\frac{\varepsilon_{\mathbf{k}} \mp a}{\sqrt{a^2+b^2+\Delta^2/4 \mp a\varepsilon_{\mathbf{k}}}}. \tag{S4}$$

The Berry connection is given by

$$\mathbf{A}(\mathbf{k}) = i\langle\psi_{\mathbf{k}}|\nabla_{\mathbf{k}}|\psi_{\mathbf{k}}\rangle = -\frac{\lambda\Delta}{4\varepsilon_{\mathbf{k}}(\varepsilon_{\mathbf{k}}-a)}\hat{z}. \tag{S5}$$

TABLE I. The quantum oscillation in nodal-line semimetals. This table shows the phase shifts measured in the experiments. $F$ distinguishes different frequencies in the samples. S means different samples. $B$ and $I$ mean the magnetic field and current directions, respectively. c and a are crystallographic axes. T means transverse conguration.

| Ref. | Sample | $B$ | $I$ | $F$ | $\phi$ |
|---|---|---|---|---|---|
| [1] | ZrSiS | T | T | 18.9 | 0 |
| | | | | 246.3 | 0.46 |
| [2] | ZrSiS | c | a | 23 | - |
| | | | | 130 | - |
| | | | | 243 | $\approx 0$ |
| [3] | ZrSiS | c | - | 8.4 | 0.16 |
| | | | | 240 | 1.21 |
| [4] | ZrSiS | c | a | 14.15 | - |
| | | | | 238.24 | 0.15 |
| [5] | ZrSiSe | c | - | 210 | 0.53 |
| [5] | ZrSiSe | in plane | - | 19.2, 22.8, 24 | nontrivial |
| | | | - | 126.9, 132.7, 142 | nontrivial |
| [5] | ZrSiTe | c | - | 102 | 0.25 |
| | | | | 154 | 0.85 |
| [6] | ZrGeS | c | - | 12.5, 236, 380 | - |
| [6] | ZrGeS | in plane | - | 17, 32 | nontrivial |
| [6] | ZrGeSe | c | - | 37.4, 226, 360 | nontrivial |
| [6] | ZrGeSe | in plane | - | 17.3, 112 and 167 | - |
| [6] | ZrGeTe | c | - | 62, 265 | nontrivial |
| [6] | ZrGeTe | in plane | - | 13, 156, 203 | nontrivial |
| [7] | HfSiS | a | - | 13.5 | 0.93 |
| | | | | 138.5 | - |
| [7] | HfSiS | c | - | 31 | 0.94 |
| | | | | 264 | 0.89 |

Therefore, the Berry curvature is

$$\Omega(\mathbf{k}) = \nabla_{\mathbf{k}} \times \mathbf{A}(\mathbf{k}) = \frac{\hbar^2 \lambda \Delta}{4m\varepsilon_{\mathbf{k}}^3}(-k_y\hat{x} + k_x\hat{y}), \tag{S6}$$

which can be converted into the cylindrical coordinates $(k, \theta, k_z)$

$$\Omega(\mathbf{k}) = -\frac{\hbar^2 \lambda \Delta}{4m\varepsilon_{\mathbf{k}}^3} k\hat{\theta}. \tag{S7}$$

Finally, in the limit $\Delta \to 0$, the Berry phase around around the nodal line can be found as

$$\phi_{\mathrm{B}} = \int\int \lim_{\Delta\to 0} \Omega(\mathbf{k}) \cdot d\mathbf{S} = \pm\pi. \tag{S8}$$

If the nodal line breaks because the conduction and valence bands are separated by finite gap $\Delta$, we can still have a Berry phase for the same integral loop as that of $\Delta = 0$, and it is given by

$$\phi_{\mathrm{B}} = \int\int \Omega(\mathbf{k}) \cdot d\mathbf{S} = \pm\pi\left(1 - \frac{\Delta}{2E_F}\right), \tag{S9}$$

which is shown in Fig. S1.

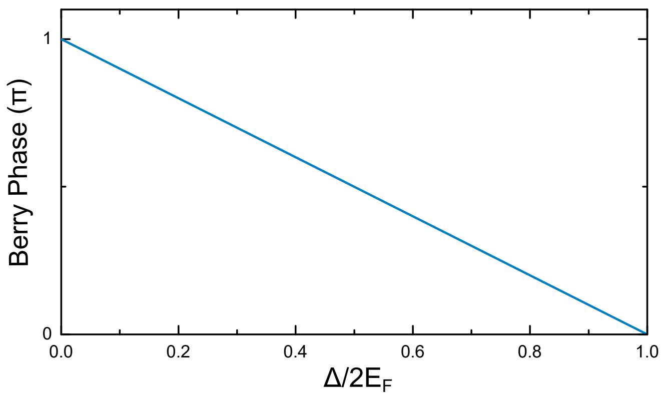


FIG. S1. The Berry phase $\phi_B$ as a function of $\Delta/2E_F$, where $\Delta$ is the gap between conduction and valence bands and $E_F$ is the Fermi energy. When $\Delta = 0$, the integral loop of the Berry phase encloses a nodal line. For a finite $\Delta$, the calculation assumes the same integral loop.

## S3. LANDAU BANDS

We apply a magnetic field along the $z$ direction, $\mathbf{B} = (0, 0, B)$, and choose the Landau gauge in which the vector potential is $\mathbf{A} = (-yB, 0, 0)$. Under the Peierls replacement, we replace the wave vector in the Hamiltonian in Eq. (2) with the operator $\mathbf{k} = (k_x - eyB/\hbar, -i\partial_y, k_z)$. By introducing the ladder operators, $a \equiv -[(y - \ell_B^2 k_x)/\ell_B + \ell_B\partial_y]/\sqrt{2}$ and $a^\dagger \equiv -[(y - \ell_B^2 k_x)/\ell_B - \ell_B\partial_y]/\sqrt{2}$, where the magnetic length $\ell_B = \sqrt{\hbar/eB}$, we have $k_x^2 + k_y^2 \to \omega(a^\dagger a + 1/2)$. Then we can rewrite the Hamiltonian as

$$H = \left[\hbar\omega\left(a^\dagger a + 1/2\right) - u\right]\tau_3 \otimes \sigma_0 + \lambda k_z \tau_1 \otimes \sigma_0, \tag{S10}$$

where $\omega = eB/m$. With the help of the trial wave function $(c_1, c_2, c_3, c_4)^T|\nu\rangle$ for $\nu = 0, 1, 2, ...$, where $\nu$ indexes the Hermite polynomials, the eigenenergies of the system in the presence of magnetic field are given by

$$E_{k_z}^{\nu\pm} = \pm\sqrt{\left[\hbar\omega\left(\nu + 1/2\right) - u\right]^2 + \lambda^2 k_z^2}, \tag{S11}$$

where $\pm$ denote the upper band and the lower band, respectively. The corresponding eigenstates are written as

$$|\nu, k_x, k_z, +\rangle = \begin{bmatrix} \cos\theta_{k_z}^{\nu+} \\ 0 \\ \sin\theta_{k_z}^{\nu+} \\ 0 \end{bmatrix} |\nu\rangle|k_x, k_z\rangle \text{ or } \begin{bmatrix} 0 \\ \cos\theta_{k_z}^{\nu+} \\ 0 \\ \sin\theta_{k_z}^{\nu+} \end{bmatrix} |\nu\rangle|k_x, k_z\rangle, \tag{S12}$$

$$|\nu,k_x,k_z,-\rangle=\begin{bmatrix}\cos\theta_{k_z}^{\nu-}\\0\\\sin\theta_{k_z}^{\nu-}\\0\end{bmatrix}|\nu\rangle|k_x,k_z\rangle \text{ or } \begin{bmatrix}0\\\cos\theta_{k_z}^{\nu-}\\0\\\sin\theta_{k_z}^{\nu-}\end{bmatrix}|\nu\rangle|k_x,k_z\rangle, \tag{S13}$$

where

$$\tan\theta_{k_z}^{\nu\pm}=\frac{\lambda k_z}{M_\nu\pm\sqrt{\lambda^2k_z^2+M_\nu^2}}, \tag{S14}$$

and $M_\nu = \hbar\omega(\nu+1/2)-u$. The wavefunctions $\psi_{\nu,k_z,k_x}(\mathbf{r})\equiv\langle\mathbf{r}|\nu,k_x,k_z\rangle$ are found as

$$\psi_{\nu,k_z,k_x}(\mathbf{r})=\frac{C_\nu}{\sqrt{L_xL_z}}e^{ik_zz}e^{ik_xx}e^{-[(y-y_0)^2/2\ell_B^2]}\mathcal{H}_\nu\left(\frac{y-y_0}{\ell_B}\right), \tag{S15}$$

where $C_\nu=1/\sqrt{\nu!2^\nu\ell_B\sqrt{\pi}}$, $L_x$ and $L_z$ are the lengths of the sample along the $x$ and $z$ directions, respectively. The guiding center $y_0=\ell_B^2k_x$, and $\mathcal{H}_\nu$ are the Hermite polynomials. The Landau degeneracy of each state is $N_L=1/2\pi\ell_B^2=eB/h$. Also, each state is 2-fold degenerate because of $\sigma_0$ in the model.

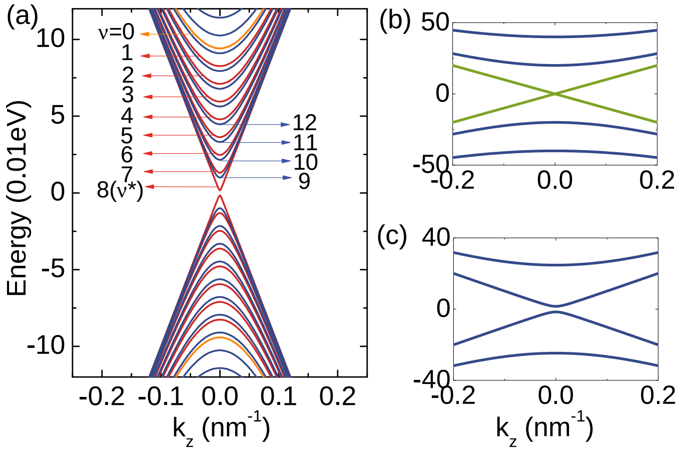


FIG. S2. (a) The Landau bands for the nodal-line semimetal in a $z$-direction magnetic field $B$, as functions of the wave vector $k_z$. The parameter are $u=0.1$ eV, $\lambda=1$ eV nm, $m=0.1m_e$, and $B=10$ T. The red lines indicate the bands with $0\le\nu\le\nu^*$, and the blue ones are for the bands with $\nu\ge\nu^*$. (b) The Landau bands at $B=172.76$ T, where the $\nu=0$ bands intersect at $E=0$. (c) The Landau bands at $B=200$ T, where the gap opens at $k_z=0$.

At different magnetic fields, there are three cases for the spectrum of the Landau bands, as shown in Fig. S2. Here we mainly discuss the electron Landau bands of positive energies since the discussion for the hole Landau bands with negative energies is similar by changing the sign from + to −. The bottoms of the electron Landau bands are at $k_z=0$.

For small magnetic field $\hbar\omega<2u$, the band bottoms can be found from Eq. (S11)

$$E_{k_z=0}^{\nu+}=\begin{cases}u-\hbar\omega\left(\nu+\frac{1}{2}\right), & 0\le\nu\le\nu^*,\\ \hbar\omega\left(\nu+\frac{1}{2}\right)-u, & \nu\ge\nu^*+1.\end{cases} \tag{S16}$$

where $\nu^*$ is the integer portion of $u/\hbar\omega-1/2$. Therefore, we can see two sets of Landau bands at low energy, as shown in Fig. S2 (a). The lowest Landau bands are shown by the orange lines with the band bottom at $u-\hbar\omega/2$. As the Landau index increases, the bands go downward. The red lines correspond to the bands with $0\le\nu\le\nu^*$. Further increasing the Landau index from $\nu^*$, the bands will go upward, as shown by the blue lines in Fig. S2 (a). This behavior is distinctly different from conventional systems and other topological semimetals, where the Landau bands always go upward with increasing Landau index. Two sets of Landau bands give rise to two oscillation frequencies in resistivities, and the upward and downward behaviors leads to different sign of the additional phase shift (−1/8 and +1/8).

The gap between the positive and negative bands is

$$\Delta=2u-2\hbar\omega(\nu^*+1/2). \tag{S17}$$

The gap closes when $u/\hbar\omega-1/2=\nu^*$ is an integer. With increasing magnetic field, the gap opens and closes back and forth. For a given $\nu^*$, the gap reaches the maximum value when $\hbar\omega=u/(\nu^*+1)$, and thus the maximum gap is found as $\Delta_{\max}=u/(\nu^*+1)$.

For $\hbar\omega=2u$,

$$E_{k_z=0}^{\nu+}=\nu\hbar\omega,\ \ \nu\ge0 \tag{S18}$$

and hence there remains only one set of Landau bands. We define this critical magnetic field $B_c$ as $2um/\hbar e$. The gap between positive and negative bands always closes. In this case the lowest Landau bands show a gapless linear dispersion

$$E_{k_z}^{0\pm}=\pm|\lambda k_z|, \tag{S19}$$

as indicated by the green lines in Fig. S2 (b).

For $\hbar\omega>2u$, there is also one set of bands, where the energies increase with the Landau index, similar to conventional systems and other topological semimetals. The gap opens and increases linearly with $B$ ($\Delta=\hbar\omega-2u$) (see Fig. S2 (c)).

For the model parameters in realistic samples, the magnetic field in the case $\hbar\omega\ge2u$ is too large in usual experimental conditions (for example, $B_c\sim172$ T in Fig. S2), so we will focus on the transport properties for the case $\hbar\omega<2u$, in which there are two sets of Landau bands.

## S4. MAGNETOCONDUCTIVITIES IN AND OUT OF THE NODAL-RING PLANE

### A. Conductivity $\sigma_{zz}$ out of the nodal-ring plane

The conductivity $\sigma_{zz}$ can be calculated as [8–10]

$$\sigma_{zz}=\frac{e^2}{k_BT}\sum_{\zeta}\tau_\zeta f(E_\zeta)[1-f(E_\zeta)](v_z^\zeta)^2, \tag{S20}$$

where $\zeta$ represents all the quantum numbers, and $f(E)=1/\{\exp[(E-E_F)/k_BT]+1\}$ is the Fermi distribution function at temperature $T$. The transport relaxation time $\tau_\zeta$ can be found by

$$1/\tau_\zeta=\sum_{\zeta'}w_{\zeta\zeta'}\left(1-v_{z\zeta'}/v_{z\zeta}\right), \tag{S21}$$

where the transition rate

$$w_{\zeta\zeta'}=\frac{2\pi}{\hbar}\langle|\langle\Psi_\zeta|V(\mathbf{r})|\Psi_{\zeta'}\rangle|\rangle^2_{\text{imp}}\delta(E_\zeta-E_{\zeta'}), \tag{S22}$$

and $\langle...\rangle_{\text{imp}}$ indicates the averaging over impurity configurations. We take the elastic impurity scattering with the potential $V(\mathbf{r})=\sum_i U(\mathbf{r}-\mathbf{R}_i)$, and impurities randomly distributing at positions $\mathbf{R}_i$.

With the expectation value for the $z$-direction velocity (defined as $\hat{v}_z\equiv(1/\hbar)(\partial H/\partial k_z)$)

$$v_z^{\pm\nu,k_z}=\pm\frac{\lambda}{\hbar}\frac{\lambda k_z}{\sqrt{M_\nu^2+\lambda^2k_z^2}}, \tag{S23}$$

Eq. (S20) at zero temperature (using $\lim_{T\to0}f(x)[1-f(x)]/k_BT=\delta(x-E_F)$) becomes

$$\sigma_{zz}=\frac{e^2}{\pi\ell_B^2}\int\frac{dk_z}{2\pi}\sum_\nu\tau_{+\nu}^{k_x,k_z}\frac{\lambda^2}{\hbar^2}\frac{\lambda^2k_z^2}{{E_F}^2}\delta(E_{k_z}^{\nu+}-E_F), \tag{S24}$$

where we have used $\sqrt{M_\nu^2+\lambda^2k_z^2}=E_F$ and the evaluation of the transport time $\tau_{+\nu}^{k_x,k_z}$ can be found from Eq. (S62) in Section S6. The summation over $\nu$ can be evaluated with the help of the Poisson integral up to the leading order

$$\sum_{\nu=0}^{\infty}F(\nu)=\frac{1}{2}F(0)+\int_0^\infty F(x)\,dx+2\sum_{k=1}^{\infty}\int_0^\infty F(x)\cos(2\pi kx)\,dx. \tag{S25}$$

Then by treating the delta function as a Gaussian form

$$\delta(x)\to\frac{1}{\delta\sqrt{\pi}}e^{-x^2/\delta^2}, \tag{S26}$$

we arrive at

$$\sigma_{zz}=\frac{2e^2}{\hbar\pi n_{\text{imp}}u_0^2}\frac{\lambda^4}{E_F^2P}\int_{-E_F/\lambda}^{+E_F/\lambda}dk_z\frac{k_z^2E_F\Pi}{\hbar\omega\sqrt{E_F^2-\lambda^2k_z^2}}, \tag{S27}$$

where $\Pi=1-2D\cos(2\pi u/\hbar\omega)\cos(2\pi\sqrt{E_F^2-\lambda^2k_z^2}/\hbar\omega)$ and $\delta$ is the broadening width. Considering $E_F\gg\hbar\omega$ and using $J_2(2\pi E_F/\hbar\omega)\approx-(1/\pi)\sqrt{\hbar\omega/E_F}\cos(2\pi E_F/\hbar\omega-\pi/4)$, where $J_\alpha$ are the Bessel functions of the first kind, we obtain

$$\sigma_{zz}=\frac{2e^2\lambda^2}{\hbar\pi n_{\text{imp}}u_0^2}\left\{1-\mathcal{C}_0D\cos\left[\frac{2\pi(u+E_F)}{\hbar\omega}-\frac{5\pi}{4}\right]-\mathcal{C}_0D\cos\left[\frac{2\pi(u-E_F)}{\hbar\omega}+\frac{5\pi}{4}\right]\right\}, \tag{S28}$$

with $\mathcal{C}_0=(2/\pi)\sqrt{\hbar\omega/E_F}$, $D=\exp[-(\pi\delta/\hbar\omega)^2]$.

### B. Conductivity $\sigma_{yy}$ in the nodal-ring plane

The conductivity $\sigma_{yy}$ can be calculated as [8–10]

$$\sigma_{yy}=\frac{e^2}{2k_BT}\sum_{\zeta\zeta'}w_{\zeta\zeta'}f(E_\zeta)[1-f(E_{\zeta'})](y_\zeta-y_{\zeta'})^2, \tag{S29}$$

The expectation value of $y$ is the guiding center, $y^{\pm\nu}=y_0$, and thus $\sigma_{yy}$ in the transverse configuration becomes

$$\sigma_{yy}=\frac{\hbar^2}{B^2}\sum_{\zeta\zeta'}w_{\zeta\zeta'}(k_x-k_x')^2\delta(E_\zeta-E_F) \tag{S30}$$

at zero temperature. For the Landau bands in nodal-line semimetals, the transition rate can be found by using Eq. (S53) and Eq. (S55)

$$w_{\zeta\zeta'}=\frac{2\pi n_{\text{imp}}u_0^2}{\hbar\Omega}\left(\cos\theta_{k_z}^{\nu+}\cos\theta_{k_z'}^{\mu+}+\sin\theta_{k_z}^{\nu+}\sin\theta_{k_z'}^{\mu+}\right)^2\times\sum_{\mathbf{q}}F_{q_\parallel}^{\mu,\nu,\nu,\mu}\delta(E_\zeta-E_\zeta')\delta_{q_z+k_z,k_z'}\delta_{q_x+k_x,k_x'}, \tag{S31}$$

where the form factor is given by

$$F_{q_\parallel}^{\mu,\nu,\nu,\mu}=e^{-u}u^{|\mu-\nu|}\left[L_{\min(\mu,\nu)}^{|\mu-\nu|}(u)\right]^2\frac{\min(\mu,\nu)!}{\max(\mu,\nu)!}, \tag{S32}$$

with $L_{\min(\mu,\nu)}^{|\mu-\nu|}(u)$ being associated Laguerre polynomials and $u=\ell_B^2q_\parallel^2/2$. We can find $\sigma_{yy}$ as

$$\sigma_{yy}=\frac{e^3n_{\text{imp}}u_0^2B}{h^2}\sum_{\nu,\mu}\sum_{k_z,k_z'}(\nu+\mu+1)\left(\cos\theta_{k_z}^{\nu+}\cos\theta_{k_z'}^{\mu+}+\sin\theta_{k_z}^{\nu+}\sin\theta_{k_z'}^{\mu+}\right)^2\delta\left(E_F-E_{k_z}^{\nu+}\right)\delta\left(E_F-E_{k_z'}^{\mu+}\right). \tag{S33}$$

This equation can be simplified as

$$\sigma_{yy}=\frac{e^3n_{\text{imp}}u_0^2B}{4h^2E_F^2}\sum_{\nu,\mu,k_z,k_z'}(\nu+\mu+1)(E_F^2+M_\nu M_\mu+2\lambda^2k_zk_z')\delta\left(E_F-E_{k_z}^{\nu+}\right)\delta\left(E_F-E_{k_z'}^{\mu+}\right), \tag{S34}$$

where the term of $2\lambda^2 k_z k_z'$ vanishes by the summation over $k_z$ and $k_z'$. Thus,

$$\sigma_{yy} = \frac{e^3 n_{\mathrm{imp}} u_0^2 B}{4h^2 E_F^2} \sum_{\nu,\mu,k_z,k_z'} (\nu+\mu+1)(E_F^2 + M_\nu M_\mu) \times \delta\left(E_F - E_{k_z}^{\nu+}\right)\delta\left(E_F - E_{k_z'}^{\mu+}\right). \tag{S35}$$

The one in the first parentheses can be dropped due to $E_F \gg \hbar\omega$. By treating the $\delta$ function to a Gaussian function, the summations over the Landau indices can be evaluated with the help of the Poisson integral, which leads to the longitudinal conductivity

$$\sigma_{yy} \approx \frac{e^3 n_{\mathrm{imp}} u_0^2 B}{\lambda^2}\frac{E_F^2 u}{\hbar^5\omega^3}\left\{\left[1 - 4D\cos\left(\frac{2\pi u}{\hbar\omega}\right) J_0\left(\frac{2\pi E_F}{\hbar\omega}\right)\right] + \frac{3E_F}{u}\sin\left(\frac{2\pi u}{\hbar\omega}\right) J_1\left(\frac{2\pi E_F}{\hbar\omega}\right)\right\}. \tag{S36}$$

For $E_F \gg \hbar\omega$, using $J_0(2\pi E_F/\hbar\omega) \approx (1/\pi)\sqrt{\hbar\omega/E_F}\cos(2\pi E_F/\hbar\omega - \pi/4)$, $J_1(2\pi E_F/\hbar\omega) \approx (1/\pi)\sqrt{\hbar\omega/E_F}\sin(2\pi E_F/\hbar\omega - \pi/4)$, we obtain

$$\sigma_{yy} = \frac{e^2 n_{\mathrm{imp}} u_0^2 m}{\lambda^2}\frac{E_F^2 u}{\hbar^5\omega^2}\left\{1 + \mathcal{C}_1 D\cos\left[\frac{2\pi(u+E_F)}{\hbar\omega} - \frac{5\pi}{4}\right] + \mathcal{C}_2 D\cos\left[\frac{2\pi(u-E_F)}{\hbar\omega} + \frac{5\pi}{4}\right]\right\}, \tag{S37}$$

where $\mathcal{C}_1 = [(4u+3E_F)/2u\pi]\sqrt{\hbar\omega/E_F}$, $\mathcal{C}_2 = [(4u-3E_F)/2u\pi]\sqrt{\hbar\omega/E_F}$.

### C. Hall conductivity $\sigma_{xy}$ in the nodal-ring plane

The Hall conductivity $\sigma_{xy}$ can be calculated as

$$\sigma_{xy} = -ie^2\hbar\sum_{\zeta\zeta'} v_x^{\zeta'\zeta} v_y^{\zeta\zeta'}\frac{f(E_{\zeta'}) - f(E_\zeta)}{(E_{\zeta'} - E_\zeta)^2}, \tag{S38}$$

where the velocity operators are $\hat{v}_x = (\hbar k_x/m - eBy/m)\tau_3 \otimes \sigma_0$ and $\hat{v}_y = (-i\hbar\partial_y/m)\tau_3\otimes\sigma_0$. With the help of the wavefunctions in Eq. (S15), the production of the velocities is found as

$$v_x^{s_1\nu,s_2\mu} v_y^{s_2\mu,s_1\nu} = \begin{cases} \frac{i\hbar^2(\nu+1)}{2m^2\ell_B^2}(\Lambda_{\nu+1,s_2}^{\nu,s_1})^2, \mu = \nu+1, \\ -\frac{i\hbar^2\nu}{2m^2\ell_B^2}(\Lambda_{\nu-1,s_2}^{\nu,s_1})^2, \mu = \nu-1. \end{cases} \tag{S39}$$

where

$$\Lambda_{\mu,s_2}^{\nu,s_1} = (\cos\theta_{k_z}^{\nu s_1}\cos\theta_{k_z}^{\mu s_2} - \sin\theta_{k_z}^{\nu s_1}\sin\theta_{k_z}^{\mu s_2})\delta_{k_x,k_x'}\delta_{k_z,k_z'}, \tag{S40}$$

and $s_1, s_2 = \pm$. Then, the Hall conductivity can be written as

$$\sigma_{xy} = \frac{\hbar^3 e^2}{\pi m^2 \ell_B^4}\sum_{k_z}\sum_\nu \frac{\nu+1}{2}\left[\frac{f(E_{k_z}^{\nu+}) - f(E_{k_z}^{\nu+1+})}{(E_{k_z}^{\nu+} - E_{k_z}^{\nu+1+})^2}(\Lambda_{\nu+1,+}^{\nu,+})^2 + \frac{f(E_{k_z}^{\nu+}) - f(E_{k_z}^{\nu+1+})}{(E_{k_z}^{\nu+} + E_{k_z}^{\nu+1+})^2}(\Lambda_{\nu+1,-}^{\nu,+})^2\right]. \tag{S41}$$

According to Eq. (S63), we further simplify the equation as

$$\sigma_{xy} = \frac{e^2}{2\pi\hbar}\sum_{k_z}\sum_\nu\left\{\frac{\nu+1}{2}\left[f(E_{k_z}^{\nu+}) - f(E_{k_z}^{\nu+1+})\right]\right\}. \tag{S42}$$

The Hall conductivity is nearly inversely proportional to the magnetic field, which has been verified numerically.

## S5. SCATTERING MATRIX ELEMENTS

In this section, we calculate the scattering matrix element $\langle U_{k_x'k_z',k_xk_z}^{\mu,\nu} U_{k_xk_z,k_x'k_z'}^{\nu,\mu}\rangle_{\mathrm{imp}}$, where [11, 12]

$$U_{k_x'k_z',k_xk_z}^{\mu,\nu} \equiv \int d\mathbf{r}'\langle\mu,k_x',k_z'|\mathbf{r}'\rangle U(\mathbf{r}')\langle\mathbf{r}'|\nu,k_x,k_z\rangle,$$
$$U_{k_xk_z,k_x'k_z'}^{\nu,\mu} \equiv \int d\mathbf{r}\langle\nu,k_x,k_z|\mathbf{r}\rangle U(\mathbf{r})\langle\mathbf{r}|\mu,k_x',k_z'\rangle. \tag{S43}$$

For simplicity, in the following we will rewrite the indices $k_x, k_z$ to $k$ and $k_x', k_z'$ to $k'$ in equations. By using

$$U(\mathbf{r}) = \sum_i \frac{1}{\Omega}\sum_{\mathbf{q}} U(\mathbf{q})e^{i\mathbf{q}\cdot(\mathbf{r}-\mathbf{R}_i)}, \tag{S44}$$

we have

$$\left\langle U_{k',k}^{\mu,\nu}U_{k,k'}^{\nu,\mu}\right\rangle_{\mathrm{imp}} = \frac{1}{\Omega^2}\sum_{\mathbf{q},\mathbf{q}'} U(\mathbf{q})U(\mathbf{q}')\left\langle\mu,k'\left|e^{i\mathbf{q}\cdot\mathbf{r}}\right|\nu,k\right\rangle \times\left\langle\nu,k\left|e^{i\mathbf{q}'\cdot\mathbf{r}}\right|\mu,k'\right\rangle\left\langle\sum_{i,j} e^{-i\mathbf{q}\cdot\mathbf{R}_i}e^{-i\mathbf{q}'\cdot\mathbf{R}_j}\right\rangle_{\mathrm{imp}}, \tag{S45}$$

where

$$\left\langle\sum_{i,j} e^{-i\mathbf{q}\cdot\mathbf{R}_i}e^{-i\mathbf{q}'\cdot\mathbf{R}_j}\right\rangle_{\mathrm{imp}} \approx n_{\mathrm{imp}}\Omega\delta_{\mathbf{q}+\mathbf{q}'}. \tag{S46}$$

Then,

$$\langle U_{k',k}^{\mu,\nu}U_{k,k'}^{\nu,\mu}\rangle_{\mathrm{imp}} = \frac{n_{\mathrm{imp}}}{\Omega}\sum_{\mathbf{q}} U(\mathbf{q})U(-\mathbf{q}) \times\langle\mu k'|e^{i\mathbf{q}\cdot\mathbf{r}}|\nu,k\rangle\langle\nu,k|e^{-i\mathbf{q}\cdot\mathbf{r}}|\mu k'\rangle, \tag{S47}$$

where

$$\langle\mu,k'|e^{i\mathbf{q}\cdot\mathbf{r}}|\nu,k\rangle = \frac{C_\mu C_\nu}{L_x L_z \ell_B}\int d\mathbf{r}e^{i\mathbf{q}\cdot\mathbf{r}}e^{i(k_z-k_z')z}e^{i(k_x-k_x')x} \times e^{-\frac{(y-y_0')^2}{2\ell_B^2}}e^{-\frac{(y-y_0)^2}{2\ell_B^2}}\mathcal{H}_\mu\left(\frac{y-y_0'}{\ell_B}\right)\mathcal{H}_\nu\left(\frac{y-y_0}{\ell_B}\right), \tag{S48}$$

$$\langle\nu,k'|e^{-i\mathbf{q}\cdot\mathbf{r}}|\mu,k\rangle = \frac{C_\nu C_\mu}{L_x L_z \ell_B}\int d\mathbf{r}e^{-i\mathbf{q}\cdot\mathbf{r}}e^{i(k_z-k_z')z}e^{i(k_x-k_x')x} \times e^{-\frac{(y-y_0')^2}{2\ell_B^2}}e^{-\frac{(y-y_0)^2}{2\ell_B^2}}\mathcal{H}_\nu\left(\frac{y-y_0'}{\ell_B}\right)\mathcal{H}_\mu\left(\frac{y-y_0}{\ell_B}\right). \tag{S49}$$

With the help of

$$\int_{-\infty}^{\infty} e^{-x^2}\mathcal{H}_m(x+y)\mathcal{H}_n(x+z)dx$$
$$= 2^n\pi^{1/2}m!z^{|n-m|}L_m^{|n-m|}(-2yz), \tag{S50}$$

and the definition of the $\delta$ function

$$\int_{-\infty}^{+\infty} dx e^{i(k-k')x} = 2\pi\delta_{kk'}, \tag{S51}$$

equation (S47) can be simplified as

$$\langle U^{\mu,\nu}_{k',k}U^{\mu,\nu}_{k,k'}\rangle_{\rm imp} = \frac{n_{\rm imp}}{\Omega}\sum_{\mathbf{q}}|U(\mathbf{q})|^2 e^{-u}\delta_{q_z+k_z,k_z'}\delta_{q_x+k_x,k_x'}$$
$$\times u^{|\mu-\nu|}L^{|\mu-\nu|}_{\min(\mu,\nu)}(u)L^{|\mu-\nu|}_{\min(\mu,\nu)}(u)\frac{\min(\mu,\nu)!}{\max(\mu,\nu)!}. \tag{S52}$$

Considering the short-range scattering $U(\mathbf{q}) = u_0$, finally we have

$$\langle U^{\mu,\nu}_{k',k}U^{\mu,\nu}_{k,k'}\rangle_{\rm imp} = \frac{n_{\rm imp}u_0^2}{\Omega}\sum_{\mathbf{q}} e^{-u}\delta_{q_z+k_z,k_z'}\delta_{q_x+k_x,k_x'}$$
$$\times u^{|\mu-\nu|}L^{|\mu-\nu|}_{\min(\mu,\nu)}(u)L^{|\mu-\nu|}_{\min(\mu,\nu)}(u)\frac{\min(\mu,\nu)!}{\max(\mu,\nu)!}. \tag{S53}$$

## S6. THE TRANSPORT TIME $\tau^{k_x,k_z}_{+\nu}$

The transport time is written as

$$\frac{\hbar}{\tau^{k_x,k_z}_{+\nu,+\mu}} = 2\pi\sum_{k_x',k_z'}\langle|U^{\nu+,\mu+}_{k_x,k_z,k_x',k_z'}|^2\rangle\left(1-\frac{v_z^{+\mu,k_z'}}{v_z^{+\nu,k_z}}\right)$$
$$\times\delta\left(E_F - E^{\mu+}_{k_z'}\right), \tag{S54}$$

where the scattering matrix elements

$$\langle|U_{k_x,k_z,k_x',k_z'}|^2\rangle = \left(\cos\theta^{\nu+}_{k_z}\cos\theta^{\mu+}_{k_z'} + \sin\theta^{\nu+}_{k_z}\sin\theta^{\mu+}_{k_z'}\right)^2$$
$$\times\langle U^{\mu,\nu}_{k_x',k_z',k_x,k_z}U^{\nu,\mu}_{k_x,k_z,k_x',k_z'}\rangle. \tag{S55}$$

According to Eq. (S53), we have

$$\langle U^{\mu,\nu}_{k_x',k_z',k_x,k_z}U^{\nu,\mu}_{k_x,k_z,k_x',k_z'}\rangle$$
$$= \frac{n_{\rm imp}u_0^2}{\Omega}\sum_{\mathbf{q}}F^{\mu,\nu,\nu,\mu}_{q_\parallel}\delta_{q_z+k_z,k_z'}\delta_{q_x+k_x,k_x'}, \tag{S56}$$

where the form factor is given in Eq. (S32).

Taking $k_z' \to k_z + q_z$ and using the cylindrical coordinate, we can rewrite Eq. (S54) as

$$\frac{\hbar}{\tau^{k_x,k_z}_{+\nu,+\mu}} = 2\pi n_{\rm imp}u_0^2\int_{-\infty}^{+\infty}\frac{dq_z}{2\pi}\left(1-\frac{v_z^{+\mu,k_z'}}{v_z^{+\nu,k_z}}\right)$$
$$\times\delta\left(E_F - E^{\mu+}_{k_z+q_z}\right)\int_0^{2\pi}\frac{d\varphi}{2\pi}\left(\cos\theta^{\nu+}_{k_z}\cos\theta^{\mu+}_{k_z'}\right.$$
$$\left.+\sin\theta^{\nu+}_{k_z}\sin\theta^{\mu+}_{k_z'}\right)^2\int_0^{\infty}\frac{q_\parallel dq_\parallel}{2\pi}F^{\mu,\nu,\nu,\mu}_{q_\parallel}. \tag{S57}$$

It is found that

$$\int_0^{\infty}\frac{q_\parallel dq_\parallel}{2\pi}F^{\mu,\nu,\nu,\mu}_{q_\parallel} = \frac{1}{2\pi\ell_B^2}. \tag{S58}$$

Therefore, we have

$$\frac{\hbar}{\tau^{k_x,k_z}_{+\nu}} = \sum_{\mu}\frac{\hbar}{\tau^{k_x,k_z}_{+\nu,+\mu}} = \frac{n_{\rm imp}u_0^2}{2\pi\ell_B^2}\left(P + \frac{Q}{E_F}M_\nu\right), \tag{S59}$$

where

$$P = \frac{E_F\pi}{2\hbar\omega\lambda} - \frac{4E_F}{\hbar\omega\lambda}D\cos\left(\frac{2\pi u}{\hbar\omega}\right)\left[\frac{\hbar\omega}{4E_F}J_1\left(\frac{2\pi E_F}{\hbar\omega}\right)\right.$$
$$\left.-\frac{\pi}{2}J_2\left(\frac{2\pi E_F}{\hbar\omega}\right)\right], \tag{S60}$$

$$Q = \frac{2E_F\pi}{\hbar\omega\lambda}D\sin\left(\frac{2\pi u}{\hbar\omega}\right)J_1\left(\frac{2\pi E_F}{\hbar\omega}\right). \tag{S61}$$

For the case in which multiple Landau bands are occupied by electrons, $E_F \gg \hbar\omega$, and $P \gg QM_\nu/E_F$, so

$$\frac{\hbar}{\tau^{k_x,k_z}_{+\nu}} = \frac{n_{\rm imp}u_0^2}{2\pi\ell_B^2}P. \tag{S62}$$

## S7. RELATION ABOUT $\Lambda^{\nu,s_1}_{\mu,s_2}$

In this Section, we demonstrate

$$\frac{(\Lambda^{\nu,+}_{\nu+1,+})^2}{(E^{\nu+}_{k_z} - E^{\nu+1+}_{k_z})^2} + \frac{(\Lambda^{\nu,+}_{\nu+1,-})^2}{(E^{\nu+}_{k_z} + E^{\nu+1+}_{k_z})^2} = \frac{1}{(\hbar\omega)^2}, \tag{S63}$$

which is used in the derivation of Hall conductivity. By the definition Eq. (S40), $(\Lambda^{\nu,s_1}_{\mu,s_2})^2$ is written as

$$(\Lambda^{\nu,s_1}_{\mu,s_2})^2 = \left(\cos\theta^{\nu s_1}_{k_z}\cos\theta^{\mu s_2}_{k_z} - \sin\theta^{\nu s_1}_{k_z}\sin\theta^{\mu s_2}_{k_z}\right)^2\delta_{k_x,k_x'}\delta_{k_z,k_z'}, \tag{S64}$$

Using Eq. (S14), and considering

$$\lambda^2k_z^2 = \left(s_1\sqrt{\lambda^2k_z^2+M_\nu^2}+M_\nu\right)\left(s_1\sqrt{\lambda^2k_z^2+M_\nu^2}-M_\nu\right), \tag{S65}$$

we can obtain

$$(\Lambda^{\nu,s_1}_{\mu,s_2})^2 = \frac{1}{2} + \frac{M_\nu M_\mu - \lambda^2k_z^2}{2s_1s_2\sqrt{\lambda^2k_z^2+M_\nu^2}\sqrt{\lambda^2k_z^2+M_\mu^2}}, \tag{S66}$$

It can be easily seen that

$$(\Lambda^{\nu,s_1}_{\mu,s_2})^2 = (\Lambda^{\nu,s_2}_{\mu,s_1})^2 = (\Lambda^{\mu,s_2}_{\nu,s_1})^2. \tag{S67}$$

Now, we calculate

$$\frac{(\Lambda^{\nu,+}_{\mu,\pm})^2}{(E^{\nu+}_{k_z} \mp E^{\mu+}_{k_z})^2} = \frac{\frac{1}{2}\pm\frac{M_\nu M_\mu-\lambda^2k_z^2}{2\sqrt{\lambda^2k_z^2+M_\nu^2}\sqrt{\lambda^2k_z^2+M_\mu^2}}}{\left(\sqrt{\lambda^2k_z^2+M_\nu^2}\mp\sqrt{\lambda^2k_z^2+M_\mu^2}\right)^2}. \tag{S68}$$

Therefore

$$\frac{(\Lambda^{\nu,+}_{\mu,+})^2}{(E^{\nu+}_{k_z} - E^{\mu+}_{k_z})^2} + \frac{(\Lambda^{\nu,+}_{\mu,-})^2}{(E^{\nu+}_{k_z} + E^{\mu+}_{k_z})^2} = \frac{1}{(M_\nu - M_\mu)^2}, \tag{S69}$$

which reduces to Eq. (S63) when $\mu = \nu + 1$.

## S8. PHASE SHIFTS IN $B_{||}$

When the magnetic field is applied in the nodal-line plane, i.e., in $B_{||}$, there are also two different extremal cross sections of the Fermi surface, the maximum ($\gamma$) and minimum ($\delta$) are shown in Fig. 1(c) of the main text, so a beating pattern in the resistivity is also expected. The minimum is the intersection of the Fermi surface and the plane $k_x = 0$. The maximum occurs somewhere between $\sqrt{2m(u-E_F)} < k_x < \sqrt{2mu}/\hbar$. The minimum consists of two identical cross sections threaded by the nodal line, so there is a $\pi$ or $-\pi$ Berry phase around the loop enclosing each of the $\delta$ cross sections, and the phase shift is $+1/8$ for electron carriers and $-1/8$ for hole carriers in the low-frequency component in $B_{||}$ (the last entry in Tab. II of the main text. In contrast, the Berry phase of the maximum $\gamma$ is trivial because it is equivalent to merging those of the two minimum $\delta$ cross sections, i.e., $\pi - \pi = 0$. Therefore, the phase shift in the high-frequency component is $-5/8$ for electron carriers and $+5/8$ for hole carriers (the 3rd entry in Tab. II of the main text).

## S9. PHASE SHIFT OF TRIVIAL BANDS

Usually in real systems, trivial and nontrivial bands coexist around the Fermi level. In this section, we derive the resistivities from trivial bands in both longitudinal and transverse configurations. Here we consider a parabolic dispersion, $H = M\left(\mathbf{k}^2 - k_w^2\right)$. The Landau bands are $E_\nu^{k_z} = (\nu+1/2)\omega_c + M(k_z^2 - k_w^2)$ for $\nu \geq 0$, where $\omega_c = 2M/\ell_B^2$.

With the help of the expectation value for the $z$-direction velocity

$$v_z^{\nu,k_z} = \frac{2M}{\hbar}k_z, \tag{S70}$$

and the relation

$$\lim_{T\to 0} f(x)[1-f(x)]/k_BT = \delta(x-E_F), \tag{S71}$$

the conductivity $\sigma_{zz}$ becomes

$$\sigma_{zz} = \frac{2e^2}{\pi\ell_B^2}\int\frac{dk_z}{2\pi}\sum_\nu \tau_\nu^{k_x,k_z}\frac{M^2}{\hbar^2}k_z^2\delta(E_\nu^{k_z}-E_F). \tag{S72}$$

The transport time for trivial bands at the Fermi energy can be found as

$$\begin{aligned}\frac{\hbar}{\tau_\nu^{k_x,k_z}} =& \frac{n_{\text{imp}}u_0^2}{\ell_B^2}\frac{1}{\sqrt{\pi}\delta k_z}\sum_\mu\int_{-\infty}^{+\infty}\frac{dq_z}{2\pi}q_z \\ &\times\exp\left[-\frac{(E_F-E_\mu^{k_z+q_z})^2}{\delta^2}\right].\end{aligned} \tag{S73}$$

After using the Poisson summation formula, it is found that

$$\begin{aligned}\sum_\mu \exp\left[-\frac{(E_F-E_\mu^{k_z'})^2}{\delta^2}\right] =& \frac{1}{2}\exp\left[-\frac{(E_F-\frac{\omega_c}{2}-Mk_z'^2)^2}{\delta^2}\right] \\ &+\frac{\delta\sqrt{\pi}}{\omega_c}+\frac{2\delta\sqrt{\pi}}{\omega_c}\sum_{k=1}^\infty\cos\left(2\pi k\frac{E_F-\frac{\omega_c}{2}-Mk_z'^2}{\omega_c}\right) \\ &\times\exp\left[-\left(\frac{\pi k\delta}{\omega_c}\right)^2\right].\end{aligned} \tag{S74}$$

Then the inversion of the relaxation time can be calculated as

$$\begin{aligned}\frac{1}{\tau_\nu^{k_x,k_z}} =& \frac{n_{\text{imp}}u_0^2}{2\pi M}\sqrt{\frac{E_F}{M}}\left\{1+\sqrt{\frac{\omega_c}{2E_F}}\sum_{k=1}^\infty\frac{(-1)^k}{\sqrt{k}}\right. \\ &\left.\times\cos\left(2\pi k\frac{E_F}{\omega_c}-\frac{\pi}{4}\right)\exp\left[-\left(\frac{\pi k\delta}{\omega_c}\right)^2\right]\right\}.\end{aligned} \tag{S75}$$

Further the $\delta$ function in Eq. (S72) can also be broadened by a Gaussian function. To the lowest order of $k$, the conductivity for $E_F' \gg \delta, \omega_c$ is given by

$$\begin{aligned}\sigma_{zz} = \sigma_0&\left\{1-\frac{\sqrt{2}}{2}\sqrt{\frac{\omega_c}{E_F'}}\cos\left[2\pi\left(\frac{E_F'}{\omega_c}-\frac{5}{8}\right)\right]\right. \\ &\left.\times\exp\left[-\frac{1}{2}\left(\frac{\pi\delta}{\omega_c}\right)^2\right]\right\},\end{aligned} \tag{S76}$$

where $E_F' = E_F + Mk_w^2$, and $\sigma_0 = 2ME_F'e^2/3\pi n_{\text{imp}}u_0^2$. The zeroth Landau band results in a $\pi$ phase shift. This result is in agreement with the textbook [13].

For the transverse conductivity $\sigma_{yy}$ of this trivial case, after some direct calculation, it is found that

$$\begin{aligned}\sigma_{yy} =& \frac{e^2n_{\text{imp}}u_0^2}{2}\frac{eB}{h}\sum_{\nu,\mu,k_z,k_z'}(\nu+\mu+1)\delta\left(E_F-E_\nu^{k_z}\right) \\ &\times\delta\left(E_F-E_\mu^{k_z'}\right).\end{aligned} \tag{S77}$$

The $\delta$ functions are broadened to the Gaussian form. To the lowest order of the oscillation, the summations are given by

$$\begin{aligned}\sum_{\nu k_z}\delta(E_F-E_\nu^{k_z}) =& \frac{1}{\pi\omega_c}\sqrt{\frac{E_F'}{M}}\left\{1-\sqrt{\frac{\omega_c}{2E_F'}}\right. \\ &\left.\times\cos\left(2\pi\frac{E_F'}{\omega_c}-\frac{\pi}{4}\right)\exp\left[-\left(\frac{\pi\delta}{\omega_c}\right)^2\right]\right\},\end{aligned} \tag{S78}$$

$$\begin{aligned}\sum_{\nu k_z}\nu\delta(E_F-E_\nu^{k_z}) =& \frac{2E_F'}{3\pi\omega_c^2}\sqrt{\frac{E_F'}{M}}\left\{1-\frac{E_c}{2E_F'}\sqrt{\frac{\omega_c}{2E_F'}}\right. \\ &\times\left[\cos\left(2\pi\frac{E_F'}{\omega_c}-\frac{\pi}{4}\right)-\frac{\pi\delta^2}{E_c\omega_c}\sin\left(2\pi\frac{E_F'}{\omega_c}-\frac{\pi}{4}\right)\right] \\ &\left.\times\exp\left[-\left(\frac{\pi\delta}{\omega_c}\right)^2\right]\right\},\end{aligned} \tag{S79}$$

with $E_c = E'_F - \omega_c/2$. The sin term in the second summation can be omitted due to $\pi\delta^2/E_c\omega_c \ll 1$. Finally, $\sigma_{yy}$ take a similar form as that in Ref. [13]

$$\sigma_{yy} = \frac{\sigma_0}{(\omega_c\tau_p)^2}\left\{1 + \frac{3\sqrt{2}}{4}\sqrt{\frac{\omega_c}{E'_F}}\cos\left[2\pi\left(\frac{E'_F}{\omega_c} - \frac{5}{8}\right)\right] \times \exp\left[-\frac{1}{2}\left(\frac{\pi\delta}{\omega_c}\right)^2\right]\right\}, \tag{S80}$$

where $\tau_p = 2\pi M^{3/2}/\left(n_{\mathrm{imp}}u_0^2\sqrt{E'_F}\right)$. In this case, the conductivity is approximately proportional to the scattering rate $w_{\zeta\zeta'}$, instead of the transport relaxation time. Hence, the oscillation part shows a $\pi$ phase shift compared with the longitudinal configuration, the phase shift is $-5/8$.


[1] X. Wang, *et al.*, "Evidence of both surface and bulk Dirac bands and anisotropic nonsaturating magnetoresistance in ZrSiS," Adv. Electron. Mater. **2**, 1600228 (2016).

[2] M. N. Ali, L. M. Schoop, C. Garg, J. M. Lippmann, E. Lara, B. Lotsch, and S. S. P. Parkin, "Butterfly magnetoresistance, quasi-2D Dirac Fermi surface and topological phase transition in ZrSiS," Sci. Adv. **2**, e1601742 (2016).

[3] J. Hu, Z. Tang, J. Liu, Y. Zhu, J. Wei, and Z. Mao, "Nearly massless Dirac fermions and strong Zeeman splitting in the nodal-line semimetal ZrSiS probed by de Haas–van Alphen quantum oscillations," Phys. Rev. B **96**, 045127 (2017).

[4] R. Singha, A. K. Pariari, B. Satpati, and P. Mandal, "Large nonsaturating magnetoresistance and signature of nondegenerate Dirac nodes in ZrSiS," Proc. Natl. Acad. Sci. USA **114**, 2468 (2017).

[5] J. Hu, *et al.*, "Evidence of topological nodal-line fermions in ZrSiSe and ZrSiTe," Phys. Rev. Lett. **117**, 016602 (2016).

[6] J. Hu, Y. L. Zhu, D. Graf, Z. J. Tang, J. Y. Liu, and Z. Q. Mao, "Quantum oscillation studies of the topological semimetal candidate ZrGeM (M=S, Se, Te)," Phys. Rev. B **95**, 205134 (2017).

[7] N. Kumar, K. Manna, Y. Qi, S.-C. Wu, L. Wang, B. Yan, C. Felser, and C. Shekhar, "Unusual magnetotransport from Si-square nets in topological semimetal HfSiS," Phys. Rev. B **95**, 121109 (2017).

[8] M. Charbonneau, K. M. Van Vliet, and P. Vasilopoulos, "Linear response theory revisited III: One-body response formulas and generalized Boltzmann equations," J. Math. Phys. **23**, 318 (1982).

[9] P. Vasilopoulos and C. M. Van Vliet, "Linear response theory revisited. IV. Applications," J. Math. Phys. **25**, 1391 (1984).

[10] C. M. Wang, H.-Z. Lu, and S.-Q. Shen, "Anomalous phase shift of quantum oscillations in 3D topological semimetals," Phys. Rev. Lett. **117**, 077201 (2016).

[11] H. Z. Lu, S. B. Zhang, and S. Q. Shen, "High-field magnetoconductivity of topological semimetals with short-range potential," Phys. Rev. B **92**, 045203 (2015).

[12] S.-B. Zhang, H.-Z. Lu, and S.-Q. Shen, "Linear magnetoconductivity in an intrinsic topological Weyl semimetal," New J. Phys. **18**, 053039 (2016).

[13] F. T. Vasko and O. E. Raichev, *Quantum Kinetic Theory and Applications: Electrons, Photons, Phonons* (Springer Science & Business Media, 2006).
